# Supplementary material for: Visibility Guided NMS: Efficient Boosting of Amodal Object Detection in Crowded Traffic Scenes
Source: arXiv:2006.08547 source file (2020-06-15)
Supplement: Supplementary file 1 [file result_table_tight_appendix.tex]

\begin{table}
  \caption{Averate Precision (AP) results of different NMS variants for instance-based object detection. Evaluation was performed on the validation splits of each dataset. Instance-level object detection benefits from combined training of both instance-based and amodal bounding boxes and thus yield slightly better results.}
  \label{tab:map_results_tight}
  \centering
\begin{tabular}{ll|rrrr|rr}
\toprule
                       &                   & Car & Truck & Bus & Pedestrian & mAP & Runtime \\ \midrule
\multirow{4}{*}{KITTI \cite{geiger2012we}} & Standard NMS      & \SI{0}{\percent}&\SI{0}{\percent}&\SI{0}{\percent}&\SI{0}{\percent}&\SI{0}{\percent}&\SI{0}{\milli\second}\\ \cmidrule{2-8}
                       & Soft NMS          &     &       &     &            &     &         \\
                       & Hybrid NMS        &     &       &     &            &     &         \\
                       & Hybrid + Soft NMS &     &       &     &            &     &         \\
\midrule
\multirow{4}{*}{VIPER \cite{richter2017playing}} & Standard NMS      &     &       &     &            &     &         \\ \cmidrule{2-8}
                       & Soft NMS          &     &       &     &            &     &         \\
                       & Hybrid NMS        &     &       &     &            &     &         \\
                       & Hybrid + Soft NMS &     &       &     &            &     &         \\
\midrule
\multirow{4}{*}{Syncapes \cite{wrenninge2018synscapes}} & Standard NMS      &     &       &     &            &     &         \\ \cmidrule{2-8}
                       & Soft NMS          &     &       &     &            &     &         \\
                       & Hybrid NMS        &     &       &     &            &     &         \\
                       & Hybrid + Soft NMS &     &       &     &            &     &         \\
\bottomrule
\end{tabular}
\end{table}
